# Supplementary material for: UtilCache: Effectively and Practicably Reducing Link Cost in Information-Centric Network
Source: arXiv:1811.05864 source file (2018-11-14)
Supplement: Supplementary file 1 [file appendix.tex]

\section{Appendix}
\appendix
%Appendix A
\section{Proof of Theorem \ref{transform}}
\label{transformproof}
% 推导过程
Since the independent variable is only $\mathbf{X_A}$, those variables in $LCM-G$ irrelevant to $\mathbf{X_A}$ become constants under A's view. Therefore, we have \eqref{GM:2}$\Leftrightarrow$\eqref{LM:2}, \eqref{GM:3}$\Leftrightarrow$\eqref{LM:3}.

Assume that $\Gamma=v_1v_2...v_s$ is the forwarding path of a local request for content $c$ generated from router $v_1$. $v_s$ can be either a serving router or edge router. In a time unit, each request like this will make $f^c_{v_1v_2}$, $f^c_{v_2v_3}$, ..., $f^c_{v_{s-1}v_s}$ increased by 1. For each link $\langle i,j\rangle$, let $f^c_{ij}=h^c_{ij}+\tilde{h}^c_{ij}$. Thus, either $h^c_{ij}$ or $\tilde{h}^c_{ij}$ is increased by 1 each time a request for $c$ passes through link $\langle i,j\rangle$.

\begin{figure}[htbp]
\centering
\includegraphics[width=0.3\textwidth]{pic/5.png}\\
\caption{Calculation of $\tilde{h}^c$ and $h^c$}
\label{cal}
\end{figure}

For each forwarding path for content $c$ (Fig.\ \ref{cal}):
\begin{itemize}
\item[-] If router $A$ is in the path, the increased request rate before $A$ is calculated into $\tilde{h}^c$, and the rest of this path is calculated into $h^c$. That is, for $\Gamma=v_1v_2...v_s$, if $v_k=A$, then $\forall 1< i\leq k$, $\tilde{h}^c_{v_{i-1}v_i}=\tilde{h}^c_{v_{i-1}v_i}+1$, and $\forall k< i\leq s$, $h^c_{v_{i-1}v_i}=h^c_{v_{i-1}v_i}+1$.
\item[-] If not, the increased request rate from $v_1$ to $v_s$ is all calculated into $\tilde{h}^c$, which means, $\forall 1< i\leq s$, $\tilde{h}^c_{v_{i-1}v_i}=\tilde{h}^c_{v_{i-1}v_i}+1$.
\end{itemize}

Let $\tilde{L}(\mathbf{X_A})=\sum\limits_{c\in\mathbf{C}}\sum\limits_{i\in\mathbf{N}}\sum\limits_{j\ In\mathbf{N}}h^c_{ij}$. Now we have:

$$\begin{matrix}G(\mathbf{x})&=&\sum\limits_{c\in\mathbf{C}}\sum\limits_{i\in\mathbf{N}}\sum\limits_{j\in\mathbf {N}}{f^c_{ij}}\\
    &=&\sum\limits_{c\in\mathbf{C}}\sum\limits_{i\in\mathbf{N}}\sum\limits_{j\in\mathbf{N}}(h^c_{ij}+\tilde{ h}^c_{ij})\\
&=&\sum\limits_{c\in\mathbf{C}}\sum\limits_{i\in\mathbf{N}}\sum\limits_{j\in\mathbf{N}}h^c_{ij}+\sum\limits_{c \in\mathbf{C}}\sum\limits_{i\in\mathbf{N}}\sum\limits_{j\in\mathbf{N}}\tilde{h}^c_{ij}\\
&=&\tilde{L}(\mathbf{x_A})+\sum_{c\in\mathbf{C}}\sum\limits_{i\in\mathbf{N}}\sum\limits_{j\in\mathbf{N }}\tilde{h}^c_{ij}
\end{matrix}$$

Obviously, the cache state of router $A$ is relevant merely to the request rate through $A$'s upstream links, for which $\tilde{h}^c_{ij}$ is constant.
Therefore, we have $min\ G(\mathbf{X})\Leftrightarrow min\ \tilde{L}(\mathbf{X_A})$.

Consider the meaning of $\tilde{L} (\mathbf{x_A})$. Evidently $\tilde{L} (\mathbf{X_A})$ represents the sum of upstream distance of all requests generated in the network.
Within 1 unit time, there are $p^c_A$ requests for content $c$ arriving at router A. Obviously $p^c_A$ is independent of $\mathbf{X_A}$, because none of A's upstream routers will forward a request back to $A$.

\begin{itemize}
\item[-] If router $A$ caches content $c$ (i.e.\ $1-X^c_A=0$), content request for $c$ arrived at $A$ will not be forward, which means its upstream distance is 0.
\item[-] If not (ie, $1-X^c_A=1$), content request for $c$ arrived at $A$ will be forwarded by $\bar{d}^c_A$ hops.
\end{itemize}

Consequently, we have $\tilde{L}(\mathbf{X_A})=\sum\limits_{c\in\mathbf{C}}p^c_A\bar{d}^c_A(1-x^c_A)=\sum\limits_{c\in\mathbf{C}}p^c_A\bar{d}^c_A-L(\mathbf{X_A})$, which means $min\ \tilde{L}(\mathbf{X_A})\Leftrightarrow max\ L(\mathbf{X_A})$.

Finally we have proved that $HCM-G$ is equivalent to $HCM-L$ under a local view.
